# Supplementary material for: Neural Set Function Extensions: Learning with Discrete Functions in High Dimensions
Source: arXiv:2208.04055 source file (2022-11-14)
Supplement: Supplementary file 1 [file appendix.tex]

\section{Primal and Dual LP: extended discussion}\label{app: primaldual}
Major elements to consider: 
\begin{itemize}
    \item domain of the cost vector
    \item constraints of the primal 
    \item domain of the LP solutions
    \item linear versus affine
\end{itemize}

\paragraph{Derivation of dual for LP and SDP? (either reference or proof)}

Consequences:
\begin{itemize}
    \item domain of decision variables
    \item constraints and probabilistic interpretation
    \item effect on which functions are being covered
\end{itemize}

To bring up: 
\begin{itemize}
    \item case where the cost is in $\mathbb{R}$, how does it affect constraints, solutions, the dual
    \item case where the cost is positive plus all of the above
    \item  case when we restrict the cost in an interval (e.g., convex closure)
    \item case where the offset $b$ is zero and relationship to submodular and base polyhedron
    \item alternative formulations like the ones presented in \cite{el2018combinatorial}
    
\end{itemize}

\section{Vector Set Function Extension Have No Bad Minima}\label{app: vector SFE proofs}

\begin{proposition}
Consider an arbitrary set function $f :2^{[n]}\rightarrow \mathbb{R}$, and corresponding vector SFE $\barf$. The following statements hold:
\begin{enumerate}
    \item $\min_{\xb\in \calX } \barf(\xb)=\min_{S \subseteq [n]} f(S) $
    \item %The minimizers of $ \barf(\xb)$ over $\xb\in [0,1]^d$ are a subset of the convex hull of  the minimizers of $ f(\xb)$ over $\xb\in \Omega$ 
    $\argmin_{\xb\in \calX} \barf(\xb) \subseteq \text{Hull}(\argmin_{\vone_S : S \subseteq [n]} f(S) )$
\end{enumerate}
\end{proposition}

%The assumptions on $f$ are  mild.Since we assume without loss of generality that $f(\emptyset)=0$, the non-negativity condition $\min_{S \subseteq [n]} f(S) < 0$  merely asserts that the minimization problem does not have the trivial solution $S=\emptyset$.

\begin{proof}
The inequality $\min_{\xb\in \calX} \barf(\xb) \leq \min_{S \subseteq [n]} f(S) $ automatically holds since $\min_{S \subseteq [n]} f(S) = \min_{\mathbf{1}_S : S \subseteq [n]} \barf(\mathbf{1}_S)$, and $\{\mathbf{1}_S : S \subseteq [n]\} \subseteq \calX$. So it remains to show the reverse. Indeed, letting $\xb \in \calX$ be an arbitrary point we have,
\begin{align*}
     \barf (\xb) &=  \mathbb{E}_{S \sim p_\xb} [f(S)] \\
     &=\sum_{S \subseteq [n]} p_\xb (S) \cdot f(S) \\
     &\geq \sum_{S \subseteq [n]} p_\xb (S) \cdot \min_{S \subseteq [n]} f ( S ) \\
     &=\min_{S \subseteq [n]} f ( S )
\end{align*} 
where the last equality simply uses the fact that $\sum_{S \subseteq [n]} p_\xb (S)=1$. This proves the first claim.

To prove the second claim, suppose that $\xb$ minimizes  $ \barf(\xb)$ over $\xb\in \calX$. This implies that the inequality  in the above derivation must be tight, which is true if and only if
\begin{align*}
p_\xb (S) \cdot  f(S) =  p_\xb (S) \cdot \min_{S \subseteq [n]} f ( S )  \quad  \text{ for all } S \subseteq [n].
\end{align*}
 For a given $S$, this implies that either $p_\xb (S)=0$ or $ f(S) = \min_{S \subseteq [n]} f ( S ) $. Since  $\xb = \mathbb{E}_{p_\xb}[ \vone_S] =  \sum_{S \subseteq [n]} p_\xb(S)\cdot \vone_S =\sum_{S: p_\xb(S) >0} p_\xb(S)\cdot \vone_S$. This is precisely a convex combination of points $\vone_S$ for which $f(S) =  \min_{S \subseteq [n]} f(S)$. Since $\barf$ is a convex combination of exactly this set of points $\vone_S$, we have the second claim.
 
 \iffalse
 
To prove that $\xb$ belongs to the convex hull of  the minimizers of $ f(\xb)$ over $\xb\in \Omega$  we must show that there are coefficients $a_S $ such that $\xb = \sum_{S \in \Omega} a_S S$ and have the properties: $a)$ $\sum_{S \in \Omega} a_S=1$, $b)$  $S \in \arg \min _{\xb \in \Omega} f(\xb)$ for all $S$ such that $a_S \neq 0$.

Property $a)$ follows since $( \sum_i a_i -1  ) \cdot \min_{\xb \in \Omega} f(\xb) = 0 $ and $ \min_{\xb \in \Omega} f(\xb) < 0$. Property $b)$ is true since $a_i \cdot  f(S_i) = a_i \cdot \min_{\xb\in \Omega} f(\xb) $ implies that either $a_i=0$ or $ f(S_i) = \min_{\xb\in \Omega} f(\xb) $.
\fi
\end{proof}

\section{Examples of Vector Set Function Extensions}\label{app: vector SFE examples}

This section redefines the vector SFEs given in Section \ref{sec: constructing vector SFEs}, and prove that they satisfy the definition of an SFEs. One of the conditions we must check is that $\barf$ is continuous and almost everywhere differentiable. A sufficient condition for continuity and almost everywhere differentiability that we shall use for a number of constructions is to show that $\barf$ is Lipschitz continuous. A very simple computation shows that it suffices to show that $\xb \in  \mapsto p_\xb(S)$ is Lipschitz continuous.

\begin{lemma}\label{prop: lipschitz}
If the mapping $\xb \in [0,1]^n \mapsto p_\xb(S)$ is Lipschitz continuous and $f(S)$ is finite for all $S$ in the support of $p_\xb$, then $\barf$ is also Lipschitz continuous. In particular, $\barf$ is continuous and almost everywhere differentiable. 
\end{lemma}

\begin{proof}
The Lipschitz continuity of  $\barf (\xb)$ follows directly from definition:
\begin{align*}
  \big |  \barf(\xb) -  \barf(\xb') \big |  &=  \bigg |\sum_{S \subseteq [n]} p_\xb(S)\cdot f(S) - \sum_{S \subseteq [n]} p_{\xb'}(S)\cdot f(S) \bigg |\\
    &=\bigg | \sum_{S \subseteq [n]} \big (p_\xb(S) - p_{\xb'}(S)\big ) \cdot f(S)  \bigg | 
    % &\leq  \sum_{S \in \Omega} \lvert p_\xb(S) - p_{\xb'}(S) \rvert \cdot \max_{S \in \Omega} f(S)  \\
    \leq  \left(2 k L \max_{S \subseteq [n]} f(S) \right) \, \cdot \| \xb - \xb' \|,  
    % =  | \Omega |\cdot L  \cdot \max_{S \in \Omega} f(S) \cdot \| \xb - \xb' \|,
\end{align*}
where $L$ is the maximum Lipschitz constant of $\xb \mapsto p_\xb(S)$ over any $S$ in the support of $p_\xb$, and $k$ is the maximal cardinality of the support of any $p_\xb$. % (note that since $\Omega$ is finite we may take $L$ to be sufficiently large that it is the Lipschitz constant for all $S \in \Omega$.
\end{proof}

In general $k$ can be trivially bounded by $2^n$, so $\barf$ is always Lipschitz. However in may cases the cardinality of the support of any $p_\xb$ is much smaller than $2^n$, leading too a smaller Lipschitz constant. For instance, $k=n$ in the case of the Lov\'{a}sz  extension.

\subsection{Lov\'{a}sz  extension.}\label{app: lovasz}

Recall the definition: $\xb$ is sorted so that $x_1 \geq x_2 \geq \ldots \geq x_d$. Then the Lov\'{a}sz  extension corresponds to taking $S_i = \{1,\ldots , i\}$, and letting $p_\xb({S_i})= x_i - x_{i+1}$, the non-negative increments of $\xb$ (where recall we take $x_{n+1}=0$). All other sets have zero probability. For convenience, we introduce the shorthand notation $a_i =p_\xb(S_i) = x_i - x_{i+1}$

\paragraph{Feasibility.} Clearly all $a_i = x_i - x_{i+1} \geq 0$, and $\sum_{i=1}^n a_i = \sum_{i=1}^n (x_i - x_{i+1}) = x_1 \leq 1$. Any remaining probability mass is assigned to the empty set: $p_\xb(\emptyset) = 1-x_1$, which contributes nothing to the extension $\barf$ since $f(\emptyset)=0$ by assumption. All that remains is to check that
$$\sum_{i=1}^n p_\xb(S_i)\cdot \vone_{S_i}= \xb.$$
For a given $k \in [n]$, note that the only sets $S_i$ with non-zero $k$th coordinate are $S_1, \ldots , S_k$, and in all cases $(\vone_{S_i})_k=1$. So the $k$th coordinate is precisely $\sum_{i=1}^k p_\xb(S_i)= \sum_{i=1}^k (x_i - x_{i+1})=x_k$, yielding the desired formula. 

\paragraph{Extension.} Consider an arbitrary $S \subseteq [n]$. Since we assume $\xb= \vone_S$ is sorted, it has the form $\vone_S= ( \underbrace{ 1,1, \ldots , 1}_{k \text{ times}}, 0, 0, \ldots 0)^\top$. Therefore, for each $j < k$ we have $a_j =  x_j- x_{j+1} = 1-1=0 $ and for each $j > k$ we have $a_j =  x_j - x_{j+1} = 0-0=0 $. The only non-zero probability is $a_k =  x_k - x_{k+1} = 1-0 =1$. So, 
$$\barf(\vone_S) = \sum_{i=1}^n a_i f(S_i) =  \sum_{i : i\neq k} a_i f(S_i) + a_k f(S_k) = 0 + 1\cdot f(S_k) = f(S)$$
where the the final equality follows since by definition $S_k$ corresponds exactly to the vector $( \underbrace{ 1,1, \ldots , 1}_{k \text{ times}}, 0, 0, \ldots 0)^\top= \vone_S$ and so $S_k=S$.

\paragraph{Differentiability.}

The Lov\'{a}sz is a well-known extension, whose properties have been carefully studied. In particular it is well known to be a Lipschitz function \cite{bach2019submodular}. However, for completeness we provide a simple proof here nonetheless.

 \begin{lemma}
 Let $p_\xb$ be as defined for the Lov\'{a}sz  extension. Then $\xb \mapsto p_\xb(S)$ is Lipschitz for all $S \subseteq [n]$.
 \end{lemma}
 
 \begin{proof}

 First note that $p_\xb$ is piecewise linear, with one piece per possible ordering  $x_1 \geq x_2 \geq \ldots \geq x_n$ (so $n!$ pieces in total). Within the interior of each piece $p_\xb$ is linear, and therefore Lipschitz. So in order to prove global Lipschitzness, it suffices to show that $p_\xb$ is continuous at the boundaries between pieces (the  Lipschitz constant is then the  maximum of the Lipschitz constants for  each linear piece). 
 
 Now consider a point $\xb$ with   $x_1 \geq  \ldots\geq x_i = x_{i+1} \geq \ldots \geq x_n$. Consider the perturbed point $\xb_\delta = \xb - \delta \bold{e}_i$ with $\delta>0$, and $\bold{e}_i$ denoting the $i$th standard basis vector. To prove continuity of  $p_\xb$  it suffices  to show that for any $S \in \Omega$ we have $p_{\xb_\delta}(S) \rightarrow p_\xb(S)$ as $\delta \rightarrow 0^+$. 
 
 There are two sets in the support of $p_\xb$ whose probabilities are different under $p_{\xb_\delta}$, namely:  $S_i = \{ 1,\ldots , i\}$ and $S_{i+1} = \{ 1,\ldots , i,  i+1\}$. Similarly, there are  two sets in the support of  $p_{\xb_\delta}$ whose probabilities are different under $p_\xb$, namely: $S'_i = \{ 1,\ldots , i-1, i+1\}$ and $S'_{i+1} = \{ 1,\ldots ,  i,  i+1\} = S_{i+1}$.
 
 So it suffices to show the convergence $p_{\xb_\delta}(S) \rightarrow p_\xb(S)$ for these four $S$. Consider first $S_i$: 
 
 $$\big |p_{\xb_\delta}(S_i) - p_\xb(S_i) \big | = \big | 0 - (x_i - x_{i+1}) \big | = 0 $$
 
 where the final equality uses the fact that $x_i = x_{i+1}$. Next consider $S_{i+1} = S'_{i+1}$: 
 
  $$\big |p_{\xb_\delta}(S_{i+1}) - p_\xb(S_{i+1}) \big | = \big |  (x'_{i+1} - x'_{i+2})  - (x_{i+1} - x_{i+2}) \big | = \big |  (x'_{i+1} - x_{i+1})  - (x'_{i+2} - x_{i+2}) \big | = 0 $$
  
  Finally, we consider $S'_{i}$:
  
   \begin{align*}
       \big |p_{\xb_\delta}(S'_{i}) - p_\xb(S'_{i}) \big | &= \big |  (x'_{i} - x'_{i+1})  - (x_{i} - x_{i+1}) \big | \\
       &= \big |  (x'_{i+1} - x_{i+1})  - (x'_{i+1} - x_{i+1}) \big | \\ 
       &=  \big |  (x_{i+1} - \delta - x_{i+1})  - (x'_{i+1} - x_{i+1}) \big |\\
       &= \delta \rightarrow 0
    \end{align*}
    
    completing the proof.
     \end{proof}

\subsection{Bounded cardinality extension.}The bounded cardinality extension coefficients $p_\xb(S)$  are the coordinates of the vector $\mathbf{y}$, where $\mathbf{y}= \mathbf{S}^{-1}\mathbf{x}$ and the entries $(i,j)$ of the inverse are
 \begin{align}
     \mathbf{S}^{-1}(i,j) = \begin{cases}
       1, \text{  if }  (j-i) \text { mod } k = 0 \text{ and } i\leq j, \\
       -1, \text{  if }  (j-i) \text { mod } k = 1 \text{ and } i\leq j, \\
       0, \text { otherwise}.
     \end{cases}
 \end{align}

\paragraph{Equivalence to the  Lova\'{s}z extension.}
We want to show that the bounded cardinality extension is equivalent to the  Lova\'{s}z extension when $k=n$.
 Let $T_{i,k}= \{j \; | \; (j-i) \text{ mod } k =0, \text{ for } i\leq j\leq n, \; j \in \mathbb{Z}_+\}$, i.e., $T_{i,k}$ stores the indices where $j-i$ is perfectly divided by $k$. From the analytic form of the inverse, observe that the $i$-th  coordinate of $\mathbf{y}$ is $p_\xb (S_i)= \sum_{j \in T_{i,k}} (x_j-x_{j+1})$. For $k=n$, we have $T_{i,n}=  \{j \; | \; (j-i) \text{ mod } n =0 \} =\{ i \}$, and therefore $p_\xb (S_i)=  x_i-x_{i+1}$, which are the coefficients of the Lovasz extension.

 \paragraph{Feasibility.} 
 The equation $\mathbf{y}= \mathbf{S}^{-1}\mathbf{x}$ guarantees that the constraint $\mathbf{x} = \sum_{i=1}^n y_{S_i} \mathbf{1}_{S_i}$ is obeyed.
Recall that $\mathbf{x}$ is sorted in descending order like in the case of the Lovasz extension. Then, it is easy to see that $p_\xb (S_i)= \sum_{j \in T_{i,k}} (x_j-x_{j+1})\leq x_i$, because $x_i-x_{i+1}$ is always contained in the summation for $p_\xb (S_i)$. Therefore, by restricting $\mathbf{x}$ in the probability simplex it is easy to see that $\sum_{i=1}^n p_\xb (S_i) \leq \sum_{i=1}^n x_i = 1 $. To secure tight equality, we allocate the rest of the mass to the empty set, i.e., $p_\xb(\emptyset)= 1-\sum_{i=1}^n p_\xb (S_i)$, which does not affect the value of the extension. \NK{make sure you check if the domain is OK}.
 
\paragraph{Extension.}
To prove the extension property we need to show that $\barf(\mathbf{1}_S) = f(S)$ for all $S$ with $|S|\leq k$.  Consider any such set $S$ and recall that we have sorted $\mathbf{1}_S$ with arbitrary tie breaks, such that $x_i=1$ for $i\leq |S|$ and $x_i=0$ otherwise. Due to the equivalence with the 
 Lova\'{s}z extension, the extension property is guaranteed when $k=n$ for all possible sets. For $k < n$,  consider the following three cases for $T_{i,k}$. 
 \begin{itemize}
     \item When $i>|S|$, $T_{i,k} = \emptyset$ because for sorted $\mathbf{x}$ of cardinality at most $k$, we know for the coordinates that $x_i=x_{i+1}=0$. For $i>k$, this implies that $p_\xb(S_i)=0$.
     \item When $i<|S|$, $\sum_{j \in T_{i,k}} (x_j-x_{j+1}) = 0$ because $x_j=x_{j+1}=1$ and we have again $p_\xb(S_i)=0$.
     \item When $i=|S|$, observe that $ \sum_{j \in T_{i,k}} (x_j-x_{j+1}) = x_i-x_{i+1} = x_i$. Therefore, $p_\xb(S_i)=1.$ in that case.  
 \end{itemize}
 Bringing it all together, $\barf(\mathbf{1}_S)= \sum_{i=1}^n p_\xb f(S_i)=  p_\xb(S) f(S) = f(S)$ since the sum contains only one nonzero term, the one that corresponds to $i=|S|$.
 
\paragraph{Differentiability.}
Similar to the Lova\'{s}z extension, $p_\xb$ in the bounded cardinality extension is piecewise linear and therefore a.e. differentiable with respect to $\mathbf{x}$, where each piece corresponds to an ordering of the coordinates of $\mathbf{x}$. On the other hand, unlike the Lova\'{s}z extension, the mapping $\mathbf{x} \rightarrow p_\xb(S)$ is not necessarily globally Lipschitz when $k < n$, because it is not guaranteed to be Lipschitz continuous at the boundaries.

\subsection{Singleton extension.}

 \paragraph{Feasibility.}

\paragraph{Extension.}
\paragraph{Differentiability.}

\subsection{Permutations and Involutory Extension.} 
 \paragraph{Feasibility.}
\paragraph{Extension.}
\paragraph{Differentiability.}

\subsection{Multilinear extension.} 

Recall that the multiliniear extension is defined via $p_\xb(S)= \prod_{i\in S }x_i \prod_{i\notin S }(1-x_i)$ supported on  all subsets $S \subseteq [n]$
 in general.
 \paragraph{Feasibility.}

 The definition of  $p_\xb(S)$ is equivalent to:
 $$p_\xb(S)= \prod_{i=1 }^n x_i^{y_i} (1-x_i)^{1-y_i}$$
 where $y_i=1$ if $i \in S$ and zero otherwise. That is, $p_\xb(S)$ is the  product of $n$ independent Bernoulli distributions. So we clearly have $p_\xb(S)\geq 0$ and $\sum_{S \subseteq [n]} p_\xb(S)= 1$. The final feasibility condition, that $\sum_{S \subseteq [n]} p_\xb(S)\cdot \vone_{S}= \xb$ can be checked by induction on $n$. For $n=1$ there are only two sets: $\{1\}$ and the empty set. And clearly $p_\xb(\{1\})\cdot \vone_{\{1\}} = x_1 (1-x_1)^{0}= x_1$, so we have the base case.

\paragraph{Extension.}

For any $S \subseteq [n]$ we have $p_{\vone_S}(S) = \prod_{i\in S }x_i \prod_{i\notin S }(1-x_i) = \prod_{i\in S }1 \prod_{i\notin S }(1-0) = 1$. So $\barf(\vone_S) = \mathbb{E}_{T \sim p_\xb} f(T) = f(S)$.
\paragraph{Differentiability.}
Fix and $S \subseteq [n]$. Again we check Lipschitzness. We use $\partial_{x_k}$ to denote the derivative operator with respect to $x_k$. If $k \in S$ we have 
$$ \abs{\partial_{x_k} p_{\vone_S}(S)} = \abs{ \partial_{x_k}\prod_{i\in S }x_i \prod_{i\notin S }(1-x_i)} = \prod_{i\in S\setminus \{k\} }x_i \prod_{i\notin S }(1-x_i) \leq 1.$$
Similarly, if $k \notin S$ we have,
$$ \abs{\partial_{x_k} p_{\vone_S}(S)} = \abs{ \partial_{x_k}\prod_{i\in S }x_i \prod_{i\notin S }(1-x_i)} = \abs{ - \prod_{i\in S }x_i \prod_{i\notin S\cup \{k\} }(1-x_i)} \leq 1.$$
Hence the spectral norm of the Jacobian $J p_\xb(S)$ is bounded, and so $\xb \mapsto p_\xb(S)$ is a Lipschitz map.

\section{Neural Set Function Extension Proofs}\label{app: neural SFE proofs}
Recall the definition of the primal LP:
\begin{align*}
     \underset{\mathbf{z},b}{\max}\{ \xb^{\top}\zb +b\}, 
    \ \text{ where } \   (\mathbf{z},b) \in \mathbb{R}^n \times \mathbb{R} \text{ and } \mathbf{1}_S ^\top \mathbf{z} +b  \leq f(S) \  \text{ for all } S \subseteq [n].  
\end{align*}
and primal SDP:
 \begin{align}
     \sup_{\mathbf{Z} 	\succeq 0, b \in \mathbb{R}} \{\text{Tr}(\mathbf{ZX}) + b\} \text{ subject to } \text{Tr}(\mathbf{1}_S \mathbf{1}_T^\top \mathbf{Z}) + b \leq f(S\cap T) \text{ for } S,T \subseteq [n].
 \end{align}

\begin{proposition}
(Containment of LP in SDP) For a given $\xb \in [0,1]^n$, let $\mathcal{P}_f$ be the polyhedron of primal LP feasible solutions, and $\mathcal{S}_f$ be the spectrahedron of primal SDP feasible solutions for $\mathbf{X} = \sqrt{\xb} \sqrt{\xb}^\top$, with square root taken entry-wise.  Then, for any $(\zb,b) \in \mathcal{P}_f \bigcap \mathbb{R}^n_{+}$, we have  $(\mathbf{Z} ,b) \in \mathcal{S}_f$ where $\mathbf{Z}=\text{diag}(\zb)$, and $\text{Tr}(\mathbf{ZX}) =\zb^\top \xb$.
\end{proposition}

\begin{proof}
We start with the feasibility claim. Suppose that $(\mathbf{z},b)$ is a feasible solution to the primal LP. We must show that $(\mathbf{Z} ,b)$ is a feasible solution to the primal SDP with $\mathbf{X} = \sqrt{\xb} \sqrt{\xb}^\top$ and where $\mathbf{Z}=\text{diag}(\zb)$.

Recall the general formula for the trace of a matrix product: $\text{Tr}(\mathbf{AB}) = \sum_{i,j} A_{ij}B_{ji}$. With this in mind, and noting that the $(i,j)$ entry of $\mathbf{1}_S \mathbf{1}_T^\top$ is equal to $1$ if $i,j \in S\cap T$, and zero otherwise, we have  for any $S,T \subseteq [n]$ that 
\begin{align*}
    \text{Tr}(\mathbf{1}_S \mathbf{1}_T^\top \mathbf{Z}) + b &= \sum_{i,j=1}^n (\mathbf{1}_S \mathbf{1}_T^\top)_{ij} \cdot \text{diag}(\zb)_{ij} + b\\
    &=\sum_{i,j \in S\cap T} (\mathbf{1}_S \mathbf{1}_T^\top)_{ij} \cdot \text{diag}(\zb)_{ij} + b \\
     &=\sum_{i,j \in S\cap T}  \text{diag}(\zb)_{ij} + b \\
      &=\sum_{i \in S\cap T}  z_i + b \\
       &=\vone_{S\cap T} ^\top \zb + b \\
       &\leq f(S\cap T)
\end{align*}
showing SDP feasibility. That the objective values agree is easily seen since:
\begin{align*}
\text{Tr}(\mathbf{ZX}) =  \sum_{i,j=1}^n \text{diag}(\zb)_{ij} \cdot \sqrt{x_i} \sqrt{x_j}  =\sum_{i=1}^n z_i \cdot \sqrt{x_i} \sqrt{x_i}  = \xb^{\top}\zb.
\end{align*}
\end{proof}

Recall the statement of the main result on constructing neural SFEs. 

\begin{proposition}
Let $\barf$ be a vector SFE of $f$. For any $\mathbf{X} \in \mathbb{S}_+^n$ consider an eigendecomposition $\mathbf{X} = \sum_{i=1}^n \lambda_i \xb_i \xb_i^\top$. Then the function $$\mathbf{X} \mapsto  \sum_{i=1}^n \lambda_i \barf(\xb_i)$$ is a neural SFE. 
\end{proposition}

\begin{proof}
The choice of coefficients $y_{S,T} = p_\xb(S,T)$ is  implicit in the definition of $\sum_{i=1}^n \lambda_i \barf(\xb_i)$. So our first detail to attend to is determining the coefficients $y_{S,T}$......

Next we must check feasibilitiy:

\begin{align}
    \mathbf{X}\preceq \sum_{S,T \subseteq [n]} y_{S , T}\mathbf{1}_{S} \mathbf{1}_{T}^\top \text{    and    } \sum_{ S, T \subseteq [n]} y_{{S,T}} = 1. 
\end{align}
\end{proof}

\section{Unsupervised Neural Combinatorial Optimization Experiments}\label{app: unsup comb}
\NK{TODOS: update straighthrough, erdos, reinforce baseline texts, add the info about the recently added datasets}

 All methods use the same GNN backbone: a combination of GAT \cite{velivckovic2018graph} and GRU graph convolutions \cite{li2015gated}. We use the Adam optimizer \cite{kingma2014adam} with initial $lr=10^{-4}$ and default PyTorch settings for other parameters \cite{paszke2019pytorch}.   We train with a fixed 60/20/20 train/test/val split and use grid search HPO over batch size $\{4,32,64\}$, number of GNN layers $\{6,10,16\}$ network width $\{64,128,256\}$. All models are trained for $200$ epochs. For the model with the best validation performance, we report the test performance and the standard deviation of performance over test graphs as a measure of method reliability. See Appendix \ref{app: unsup comb} for further details. 
 
\paragraph{Discrete Objectives.}
For the maximum cut objective, since we are training with gradient descent, we minimized
\begin{align}
    f_{cut}(S;G) = -\text{cut}(S;G),
\end{align}
where $S$ is an input set. It should be noted that the Lova\'{s}z extension of the cut function on a graph, corresponds to the graph total variation. For the maximum clique problem, we select the discrete objective that yielded the most stable results across datasets. It is defined as 
\begin{align}
    f_{clique}(S;G) = -w(S)q^{2}(S), \label{eq:clique_objective}
\end{align}
where $q(S)=2w(S)/(|S|^{2}-|S|))$ and $w(S) = \sum_{(i,j) \in E}{w_{ij}p_ip_j}$.

\subsection{Baselines.}
\paragraph{Erdos Goes Neural \cite{karalias2020erdos}.}We compare with recent work on unsupervised combinatorial optimization. We use the official implementation of the code and the corresponding loss function for the maximum clique problem.

For the maximum cut problem, we use the probabilistic methodology described in the paper to derive a loss function. The resulting loss for an input graph $G$ and learned probabilities $\mathbf{p}$ is
\begin{align}
    L_{\text{maxcut}}(\mathbf{p};G) = a- \E{[\text{cut(S)}]} = a-\sum_{i\in V} p_id_i + \sum_{(i,j) \in E}{w_{ij}p_ip_j},
\end{align}
where $a$ is an upper bound on the size of the optimal solution, which we omit in practice as it does not affect the optimization. 
In the original implementation, the code makes use of randomization in the input of the neural network. Specifically, each set of probabilities $\mathbf{p} \in [0,1]^{|V|}$ is computed as $f(\delta_{i};G)=\mathbf{p}$, where $\delta_{i} \in [0,1]^{|V|}$ is a one hot encoding of a randomly chosen node $i$. This allows for different sets of probabilities  conditioned on different inputs to be produced for each graph. Then each set is decoded with the method of conditional expectation into discrete outputs.
In order to ensure accurate comparisons, we only apply the method of conditional expectation on just one set of probabilities produced from one randomly generated input. Our implementation of the Lova\'{s}z extension just picks the best level set in the support of $p_\mathbf{x}$
so this establishes a level playing field for the comparisons.

\paragraph{Straight Through Estimator.}We also compared with the Straight-Through gradient estimator \citep{bengio2013estimating}. This estimator can be used to pass gradients through samples from a distribution, by assuming in the backward pass that the sampling operation is the identity. In order to obtain a working baseline with the straight-through estimator, we opted for a distribution of level sets induced by the output of a neural network. Specifically, given $\mathbf{x} \in [0,1]^{|V|}$ outputs from a neural network, we sample indicator vectors $\mathbf{1}_{S_{k}}$, where $S_{k} = \{x_j | x_j \geq  t_k \}$ where $t_k \in [0,1]$ is a randomly chosen threshold. 
Then our loss function was computed as
\begin{align}
L(\mathbf{x};G) =   \frac{1}{K}\sum_{k=1}^{K} f(\mathbf{1}_{S_{k}}),
\end{align}
where $f$ was the clique or the cut functions used in the Lova\'{s}z setting, and $K$ the total number of samples, which we set to 100.
This can be viewed as a differentiable stochastic estimate of the Lovasz extension. It should be noted that this use of the Straight-Through estimator is bound to fail for a general non-differentiable black box $f$, as no gradients will be able to flow in the backward pass. Furthermore, we have also experimented with different variants of the score function estimator. However, it demonstrated extremely unstable behavior during training and was unable to converge. As it can be seen in figures 6 and 7, our extension minimizes the loss easily across epochs, but the rewards remain unstable during training for the estimator.

We also reported results for greedy heuristics on both combinatorial problems. These are both heuristics provided with the NetworkX package 
\citep{hagberg2008exploring}. For the max-cut, the heuristic begins with an empty set and adds at each step the node that maximally increases the cut. For the max-clique heuristic, the implementation relies on an approximate indepedendent set heuristic that utilizes subgraph exclusion
\citep{boppana1992approximating}.

%  \begin{figure*}[t] %{6.5cm}
%   \begin{center}
%     \includegraphics[width=0.4\textwidth]{figs/score.pdf}
%       \vspace{-15pt}
%     \caption{Score function estimator reward over 100 epochs on maximum clique.}
%     \label{fig: k clique}
%   \end{center}
%   \vspace{-10pt}
% \end{figure*}

%  \begin{figure*}[t] %{6.5cm}
%   \begin{center}
%     \includegraphics[width=0.4\textwidth]{figs/lovasz_plot.pdf}
%       \vspace{-15pt}
%     \caption{Lova\'{s}z extension loss over 100 epochs.}
%     \label{fig: k clique}
%   \end{center}
%   \vspace{-10pt}
% \end{figure*}

\paragraph{Ground truths.}  We obtain ground truths for all our datasets and for each combinatorial problem by expressing it as a mixed integer program and solving it in Gurobi \citep{gurobi}.

\paragraph{Implementation details and datasets.} We conduct our experiments using the Pytorch Geometric API (PyG) \citep{Fey/Lenssen/2019}. The datasets PROTEINS, ENZYMES, and IMDB-Binary are part of the TUDatasets collection of graph benchmarks \citep{Morris+2020} available through the PyG API.
For our models, we use as input features the node degrees, followed by a Graph Isomorphism Network (GIN) layer \citep{xu2018powerful} and multiple iterations of the Gated Graph Convolution layer \citep{yujia2016gated}. 
We tune the width (64-256), the iterations (3-12), the learning rate (0.00001,0.001) and the batch size (4,128) of our models with a grid search over fixed values in the reported intervals. We train for 500 epochs and report the test performance of the model with the best validation score.

\subsection{Constraint satisfaction problems}

\paragraph{Ground truths.}  As before, we obtain ground truths for all our datasets and problems by expressing it as a mixed integer program and using the Gurobi solver \citep{gurobi}.

\paragraph{Implementation details and datasets.} Again we use the Pytorch Geometric API (PyG) \citep{Fey/Lenssen/2019} and access the datasets through TUDatasets collection of graph benchmarks \citep{Morris+2020} available through the PyG API. For the model architecture we use a single GAT layer \citep{velivckovic2018graph} followed by  multiple gated graph convolution layers to extract features $\xb = g(G) \in [0,1]^{|V|}$, where $\xb$ contains a single value in $[0,1]$ for each node.  We use the following same set function as we did for max-clique,
\begin{align*}
    f_{clique}(S;G) = -w(S)q^{2}(S).
\end{align*}

For both the Lov\'{a}sz  extension and $k$-subset extension, we perform an exhaustive grid search over the following hyper parameters: learning rate $lr = \{ 0.00001, 0.00005,  0.0001\}$, GNN widths $w \in \{64, 128\}$, batch size $bs \in \{32, 64, 128\}$, and depths $d \in \{8, 10\}$. Finally, we use the correction technique for improper NFEs described in Section \ref{sec: constructing proper NFE}, in which we optimize a penalization of the improper extension:

$$ w \cdot \barf(\xb) + (1-w) \cdot \beta $$

where  recall that $\xb' \defeq \E_{S \sim p_\xb}[\vone_S \big ] \neq \xb$ and we define $w \defeq \min \big ( \{{x_i}/{x'_i}\}_{i=1}^d \cup \{1\} \big )$.
We also tune the penalty $\beta$ during HPO, searching over the two values $\beta \in \{ 10,15\}$.

After completing the exhaustive grid search, we select the single model that achieves the highest F1-score on a validation set, and report as the final result the F1-score of that same model on a  separate test set.

\section{Directly minimizing training error}\label{app: image classification}

Recall that for  a $K$-way classifier $h : \mathcal X \rightarrow \mathbb{R}^K$ with 
$\hat{y}(x) = \arg \max_{k =1,\ldots, K} h(x)_k$, we consider the training error  $$\frac{1}{n}\sum_{i=1}^n \mathbf{1}\{ y_i \neq \hat{y}(x_i)\}$$  calculated over a labeled training dataset $\{(x_i,y_i)\}_{i=1}^n$ to be a discrete non-differentiable loss. The set function in question is $y \mapsto \mathbf{1}\{ y_i \neq y\}$, which we relax using the singleton method described in Section \ref{sec: examples}.

\paragraph{Training details.} For all datasests we use a standard ResNet-18 backbone, with a final layer to output a vector of the correct dimension.  All models are trained for 200 epochs, except for on SVHN, which we uses only 100. We use SGD with momentum $mom=0.9$ and weight decay $wd=5 \times 10^{-4}$ and a cosine learning rate schedule. We tune the learning rate for each loss via a simple grid search of  the values $lr \in \{ 0.01, 0.05, 0.1, 0.2\}$. For each loss we select the learning rate with highest accuracy on a validation set, then report the average accuracy on a test set  over three separate runs.
